# Supplementary material for: Rapid stellar and binary population synthesis with COMPAS
Source: arXiv:2109.10352 source file (2021-12-28)
Supplement: Supplementary file 1 [file appendix.tex]

\section{Calculating the MSSFR merger distributions and rates}
\label{sec:app-calculating-merger-distributionsMSSFR}

To calculate the DCO merger rate that is detectable with ground-based gravitational-wave interferometers today we follow a similar derivation as in e.g.  \citet{2013ApJ...779...72D, 2015ApJ...806..263D,2016ApJ...819..108B,2016MNRAS.458.2634M, 2019MNRAS.482..870E, 2019PhRvD.100f4060B,2019arXiv190612257B, 2019MNRAS.482.5012C}. The rate of DCO mergers as a function of merger time \tmerger which can be calculated by a convolution $``{*}``$ of the metallicity-specific star formation rate (MSSFR) with the formation rate of DCO mergers:

\begin{align}
	\rate_{\rm{m}} (\tmerger) &= 
		\frac{\diff^4 \Nmerger }{\diff \ts \diff \Vc  \diff \monef \diff \mtwof}
		 (\tmerger) 
		= \int \diff Z 
				\left(  
				{\SFRD} \ 
				{*}  \ 
		 		\frac{\diff^4 \Nform}{\diff \MSFR \diff \tdelay  \diff \monef \diff \mtwof}  
		  \right)
		  (\tmerger) \notag \\
		&= \int \diff Z 
		 \int_0^{\tmerger} 
		 \diff \tdelay \, 
		{{\text{SFRD}\ensuremath{(Z_{\rm{i}},z(\tform))}\xspace}} \, \times 
%		\, \hspace{4cm} 
		\rate_{\rm{form}}(Z, \tdelay, \monef, \mtwof)  
\label{eq:app-merger-rate}
\end{align}
where we used that $\tform = \tmerger - \tdelay$ where $\tform$ is the time in the Universe at which the binary was formed, and $\tdelay = \tevolve + \tinspiral$ is the time it takes the binary from formation to merge.  

The \SFRD is the metallicity-specific star formation rate, which is obtained from  
combining a SFRD  and  metallicity probability density function 
\begin{align}
	&{\rm{SFRD}}(\Zi, z_{\rm{form}}) = 
	\frac{\diff^3 \MSFR}{\diff \ts \diff \Vc \diff \Zi}(z_{\rm{form}})  
	 = \underbrace{\frac{\diff^2 \MSFR}{\diff \ts \diff \Vc }(z_{\rm{form}})}_\text{SFRD} 
	 \times 
	 \underbrace{\frac{\diff P }{\diff \Zi}(z_{\rm{form}})}_\text{GSMF $+$ MZR}, 
\end{align}

see Section~\ref{sec:postprocessing} for more details. 

% \begin{align*}
% %
% {\rm{SFR}}(z)  =   \frac{\diff^2 \MSFR}{\diff \ts \diff \Vc} = a \frac{(1+z)^b}{1+ [(1+z)/c]^d}   \ \Msun \yearmin \MpcminThree 
% %
% \end{align*}
% %
% and 
% %
% \begin{align}
% \frac{\diff \MSFR }{\diff Z}(z) = \frac{1}{Z \sigma \sqrt{2 \pi}} \exp^{-\frac{(\log_{10}(Z) - \mu(z))^2}{2 \sigma^2}}.
% \end{align}
% %

In the end we can then calculate the observed merger rate by using 
\begin{align*}
\rate_{\rm{det}}(\tdet, \monef, \mtwof) 
= \frac{\diff^3 \Ndet}{\diff \tdet  \diff \monef \diff \mtwof}   
= \int \diff \Vc  \, 
\frac{\diff \ts}{\diff \tdet}  \, 
 \rate_{\rm{m}}(\tmerger) \,  
 \Pdet (\monef, \mtwof, \DL(z)).
\end{align*}
Using the substitution $\diff \Vc =  \frac{\diff \Vc}{\diff z} \diff z $ we obtain the integral over redshift
\begin{align}
\rate_{\rm{det}}(\tdet, \monef, \mtwof) = 
	\int_0^{z_{\rm{max}}}  \diff z   \, 
	\frac{\diff \ts}{\diff \tdet}(z)  \, 
	\frac{\diff \Vc}{\diff z}(z) \,
	 \rate_{\rm{m}}(z(\tmerger)) \,  
	\Pdet (\monef, \mtwof, \DL(z)).
\label{eq:Rdet-full-integral-form2}
\end{align}

Using the relationship between source and detector frame from, e.g.,  \citealt{1999astro.ph..5116H})

\begin{align*}
\frac{\diff \ts}{\diff \tdet} = \frac{1}{(1+z)},
\end{align*}
we can then  translate the source frame time $\ts$ to the detector frame using 
\begin{align*}
\frac{\diff \Vc}{\diff z}(z)  = \frac{4 \pi c}{\Hubble} \frac{\Dc^2(z)}{E(z)}
\end{align*}
with  $\Dc(z) = \frac{c}{\Hubble} \int_0^{z} \frac{ \diff z'}{E(z')} $   and  $E(z) = \sqrt{\Omega_{\rm{m}}(1+z)^3 + \Omega_{\Lambda}}$. \\

Using that $\Pdet$ is a function dependent on \DL, which can be rewritten as: $\DL(z) = \Dc(z) (1+z)$, we can obtain  together with Eq.~\ref{eq:app-merger-rate} for the merger rate the equation 
\begin{align}
	&\rate_{\rm{det}}(\tdet, \monef, \mtwof)  = 
	\int_0^{z_{\rm{m, max}}}  \diff z_{\rm{m}}  \,  \int  \diff Z \,  \int_0^{\tmerger}  \diff \tdelay \, \frac{1}{1 + z}   {\rm{SFRD}}(\Zi,z(\tform= \tmerger(z_{\rm{m}}-\tdelay)) \times \notag \\
	&\hspace{4cm}
	\rate_{\rm{form}}(\Zi, \tdelay, \monef, \mtwof)  
	\frac{4 \pi c}{\Hubble} 
	\frac{\Dc^2(z)}{E(z)} 
	\Pdet (\monef, \mtwof, \DL(z)) 
\label{eq:Rdet-full-integral-form}
\end{align}

Since we simulate only a fixed amount of metallicities, we approximate the integral in Eq.~\ref{eq:Rdet-full-integral-form} with the Monte Carlo estimate

%\begin{widetext}
\begin{equation}\label{eq:Upsilon}
    \boxed{
	\begin{aligned}
	\rate_{\rm{det}}  =  
	\sum_{z_{{\rm{m}}}^j} \sum_{\Zi^k} \, 
	 \left( 
	 	\int_0^{\tmerger^j} \, %\tmerger(z_{{\rm{m}}}^j)
	 	 \diff \tdelay \, 
		 \rate_{{\rm{form}}}(\Zi^k, \tdelay, \monef, \mtwof)   \,
		 {\rm{SFRD}}(\Zi, z_{\rm{form}})   
	 \right) 
	   \frac{\Dc^2(z_{{\rm{m}}}^j) }{E(z_{{\rm{m}}}^j) }
	 \frac{1}{1 + z_{{\rm{m}}}^j}
 	 \frac{4 \pi c}{\Hubble} \
	  P_{{\rm{det}} }(\monef, \mtwof,z_{{\rm{m}}}^j) \,
	  \Delta z_{{\rm{m}}}^j \,
	  \Delta  \Zi^k, 
	\end{aligned}
    }
\end{equation}
%\end{widetext}

With \COMPAS we can now calculate this integral by summing over equally divided  redshift bins $z_{{\rm{m}}}^j \in [0, z_{\rm{max}}]$.  For the maximum redshift one can choose something like $z_{\rm{max}} = 2$, which is a conservative upper limit for the maximum redshift ($z=2$ is equal to $D_{\rm{L}}\approx 1.5 \cdot 10^4$) out to which DCO mergers are detectable with the LVK gravitational-wave network \citep[see Fig 3 of][]{2016PhRvD..93k2004M} and see \citet{2018LRR....21....3A}. 
This equation  also sums over our the different initial metallicity bins  $\Zi^k \in [Z_{\rm{min}}, Z_{\rm{max}}]$ that are simulated with \COMPAS.
The  $\tmerger^j$ is a short hand notation for $\tmerger(z_{{\rm{m}}}^j)$, the merger time at redshift $z_{{\rm{m}}}^j$, and 	the short hand notation  $ \Delta z_{{\rm{m}}}^j  = (z_{{\rm{m}}}^{j+1} - z_{{\rm{m}}}^j)$ and  $\Delta  Z^k = (Z^{k+1} - Z^{k})$. 
We also use $z_{\rm{form}}$ as a short hand notation for $z(\tform = \tdelay - \tmerger^j)$.  
\Dc and $E$ are functions of redshift given in Eq. C3 and C4)  and  $\Hubble$ is the Hubble constant at redshift $z=0$.
